# Supplementary material for: Towards Equitable Representation in Text-to-Image Synthesis Models with the Cross-Cultural Understanding Benchmark (CCUB) Dataset
Source: arXiv:2301.12073 source file (2023-04-26)
Supplement: Supplementary file 1 [file appendix.tex]

\subsection{Western Bias}

The dataset used to train Stable Diffusion has a known bias towards generating images containing Western content~\cite{birhane2021stereotypesInLAION}. We conducted a study to compare the images generated by Stable Diffusion versus our approach in terms of their Western appearance. We compared our model trained on the United States CCUB data and found that 72\% of our approach's generated images appeared more Western than Stable Diffusion based on 12 participants from the USA and 218 image comparisons.

% \begin{table}[]
% \centering
% \begin{tabular}{c|cc} &
%   \begin{tabular}[c]{@{}c@{}}Stable Diffusion\\ (Baseline)\end{tabular} &
%   \begin{tabular}[c]{@{}c@{}}USA Culturally-aware\\ Stable Diffusion\\ (Ours)\end{tabular} \\ \hline
% \# of Answers &
%   60 &
%   158  \\
% Percentage &
%   28\% &
%   72\%  \\ \hline
% \end{tabular}
% \caption{Results of the survey measure the differences between our American Culturally-Aware Stable Diffusion and the baseline, in terms of which method generates more Western-style images. The results shows the number and percentage of preference.}
% \label{tab:Western_compare}
% \end{table}
